# Supplementary material for: Understanding the Role of Adaptivity in Machine Teaching: The Case of Version Space Learners
Source: arXiv:1802.05190 source file (2018-12-09)
Supplement: Supplementary file 1 [file 10.6_appendix_lattice_alg.tex]

\section{\lattice: Algorithmic Details} \label{app:lattice}
In this section, we specify the \lattice hypothesis class, and present the details of the adaptive algorithm \adalteacher (which is used to instantiate \adal from \algref{alg:non-myopic}) and the non-adaptive algorithm \nonadar, and provide the proof for \lemref{lm:lattice}.

\subsection{Preference Structure and The Greedy Teacher}

\paragraph{Preference function}
% \yuxin{redefine distances}
Recall that hypotheses in \lattice are represented by its nodes, and the preference function is defined through the $L_1$ distance: $\orderingof{h'}{h} = L_1(h',h)$. To facilitate understanding of the concept class, one can imagine a toy scenario, where the teacher aims to teach/steer a human learner to reach a goal state in a physical environment. Each hypothesis/node corresponds to some unexplored territory, and there exists an example which flags the territory as explored. The learner prefers local moves, and if all neighboring territories are explored, the learner jumps to the next closest one.

% Recall that hypotheses in \lattice are represented by its nodes, and the preference function is defined through $\tilde{D}$ (Eq.~\eqref{eq:objrank}): the ones that are closer to the target hypothesis measured by $\futurecostapprox(\hypothesis, \Hypotheses_t, \hstar)$) are more preferred. To facilitate understanding of the concept class, one can imagine a toy scenario, where the teacher aims to teach/steer a human learner to reach a goal state in a physical environment. Each hypothesis/node corresponds to some unexplored territory, and there exists an example which flags the territory as explored. The learner prefers local moves, and if all neighboring territories are explored, the learner jumps to the next closest one.

\paragraph{A failure case for the myopic adaptive teaching algorithm} We show in \figref{fig:app:lattice} that the myopic teacher w.r.t. Eq.~\eqref{eq:objrank} can perform poorly on simple teaching tasks. As we can see in the first plot of \figref{fig:app:lattice:myopic}, the learner starts at square $\hinit = (2,2)$ and the target hypothesis is at $\hstar = (4,4)$. The target hypothesis is the least preferred hypothesis from $\hinit$. Any teaching example will not change the rank of $\hstar$:
\begin{itemize}
\item Any example other than $(2,2)$ will not move the learner away from $\hinit$, hence the gain in $\futurecostapprox(\hinit, \Hypotheses)$ is 1.
\item Meanwhile, the teaching example $(1,1)$ moves the learner away from $(1,1)$. However, when computing the greedy heuristic we are considering the gain in the worst-case---which corresponds to the case where the learner jumps to $(1,2)$ or $(2,1)$, and the gain is 1.
\end{itemize}
In this particular example, the gradient of the objective function (Eq.~\eqref{eq:objrank}) is 0, which provides no information as to which example to select next. Hence, the myopic teacher uses random instances to teach; in the worst case, the performance can be arbitrarily bad, even compared with a non-adaptive policy.

% Next, we provide an example where the myopic teacher \algref{alg:myopic} performs poorly.

\begin{figure*}[!ht]
  \centering
  \begin{subfigure}[b]{1.0\textwidth}
    \includegraphics[trim={8pt 5pt 8pt 5pt},height=.11\textwidth]{./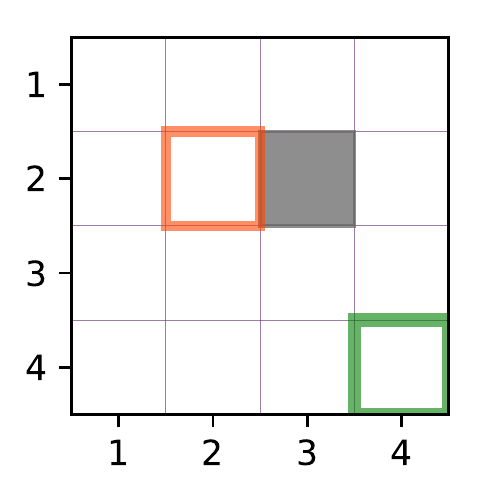}
    \includegraphics[trim={8pt 5pt 8pt 5pt},height=.11\textwidth]{./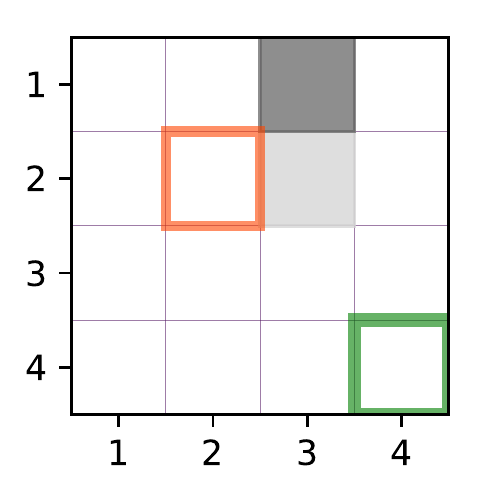}
    \includegraphics[trim={8pt 5pt 8pt 5pt},height=.11\textwidth]{./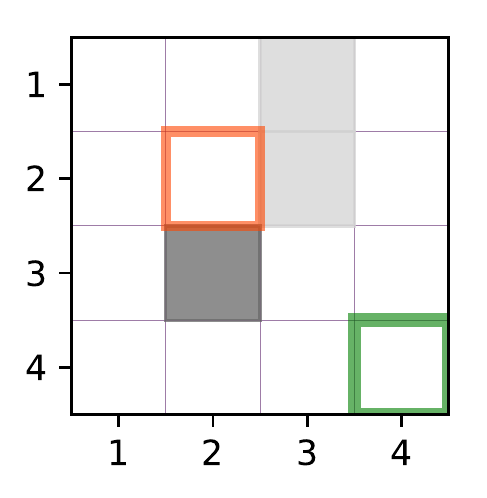}
    \includegraphics[trim={8pt 5pt 8pt 5pt},height=.11\textwidth]{./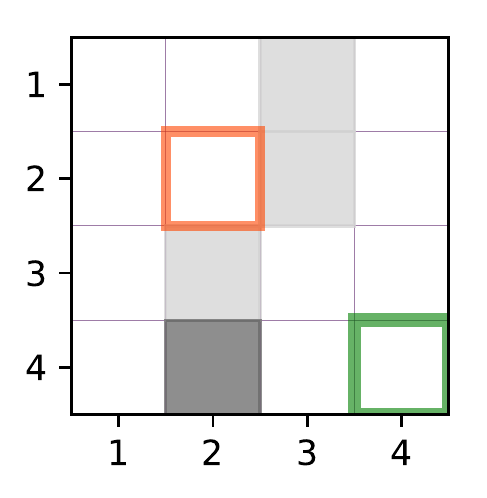}
    \includegraphics[trim={8pt 5pt 8pt 5pt},height=.11\textwidth]{./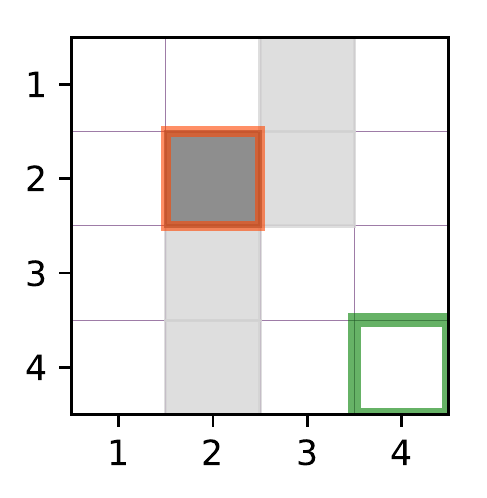}
    \includegraphics[trim={8pt 5pt 8pt 5pt},height=.11\textwidth]{./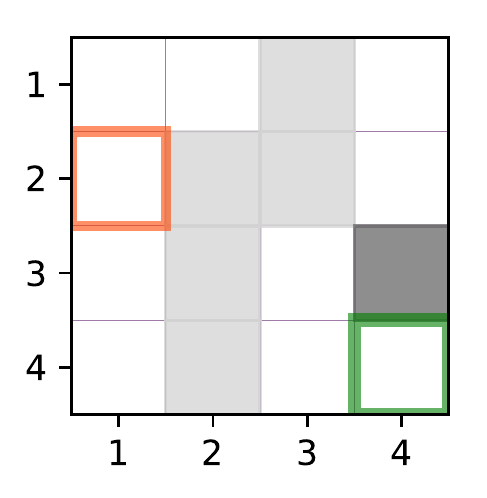}
    \includegraphics[trim={8pt 5pt 8pt 5pt},height=.11\textwidth]{./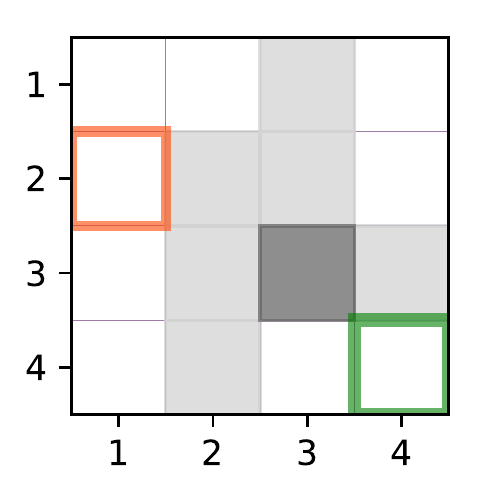}
    \includegraphics[trim={8pt 5pt 8pt 5pt},height=.11\textwidth]{./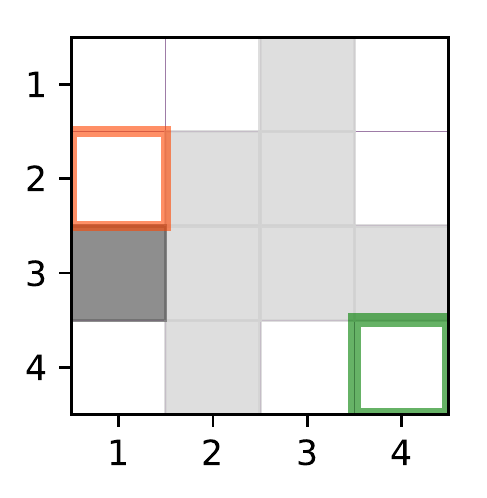}
    \includegraphics[trim={8pt 5pt 8pt 5pt},height=.11\textwidth]{./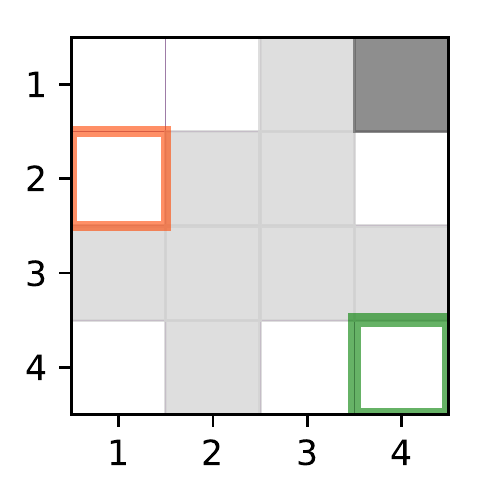}
    \caption{Myopic algorthim w.r.t. Eq.~\eqref{eq:objrank}}
    \label{fig:app:lattice:myopic}
  \end{subfigure}
  \begin{subfigure}[b]{1.0\textwidth}
    \includegraphics[trim={8pt 5pt 8pt 5pt},height=.11\textwidth]{./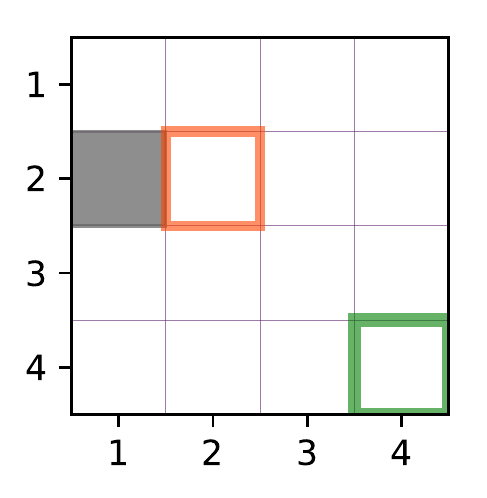}
    \includegraphics[trim={8pt 5pt 8pt 5pt},height=.11\textwidth]{./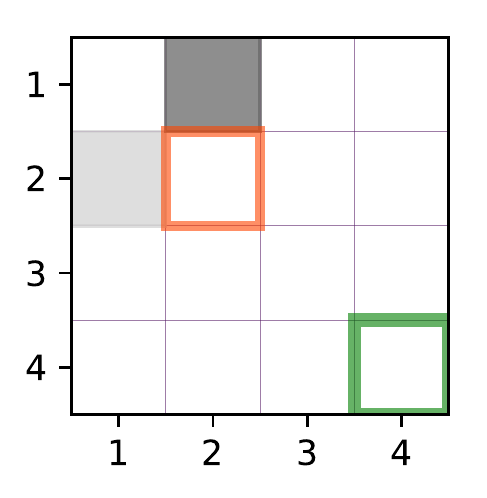}
    \includegraphics[trim={8pt 5pt 8pt 5pt},height=.11\textwidth]{./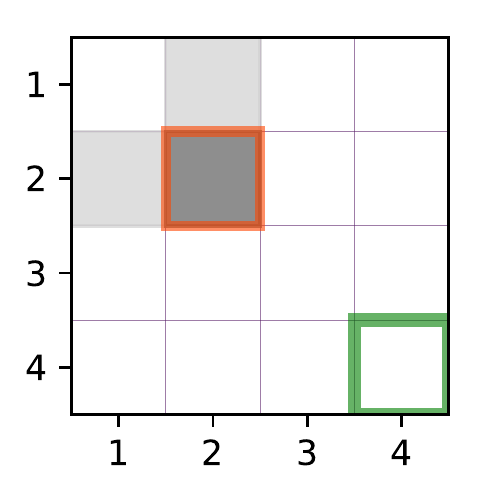}
    \includegraphics[trim={8pt 5pt 8pt 5pt},height=.11\textwidth]{./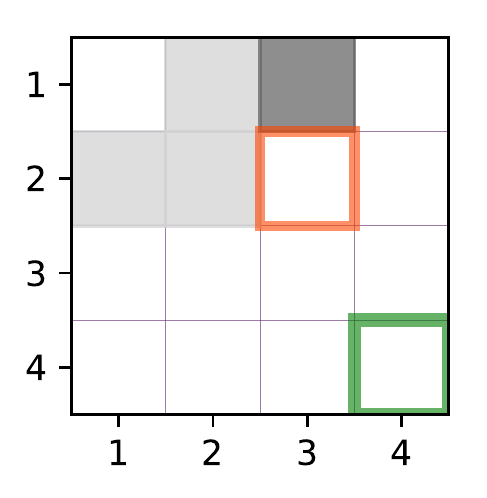}
    \includegraphics[trim={8pt 5pt 8pt 5pt},height=.11\textwidth]{./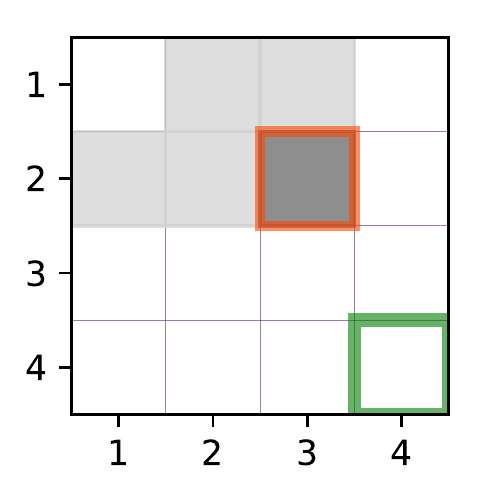}
    \includegraphics[trim={8pt 5pt 8pt 5pt},height=.11\textwidth]{./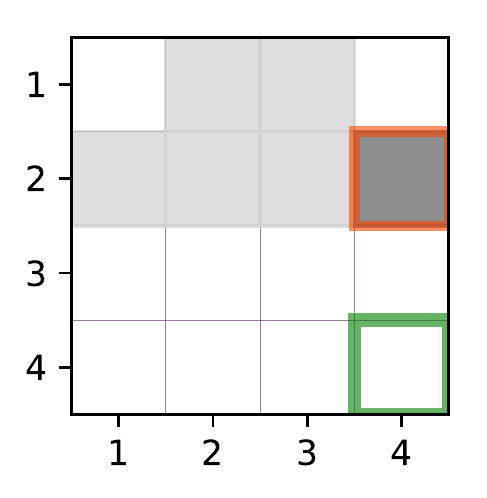}
    \includegraphics[trim={8pt 5pt 8pt 5pt},height=.11\textwidth]{./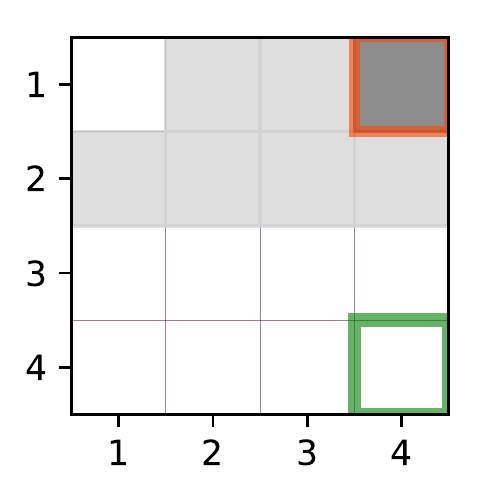}
    \includegraphics[trim={8pt 5pt 8pt 5pt},height=.11\textwidth]{./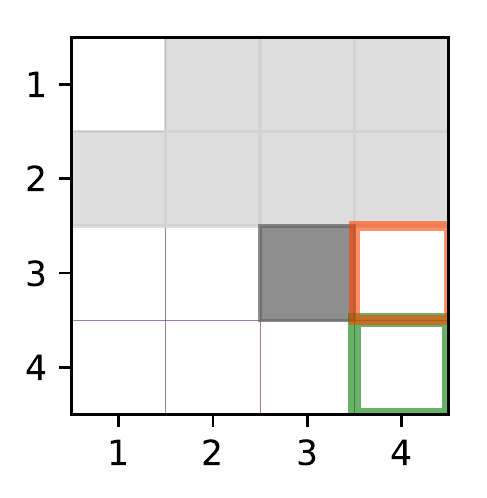}
    \includegraphics[trim={8pt 5pt 8pt 5pt},height=.11\textwidth]{./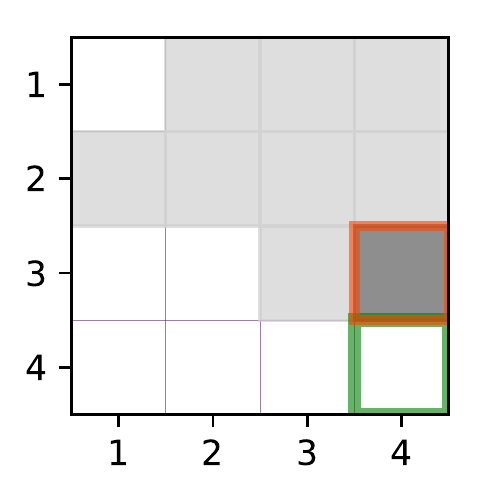}
    \caption{\adal -- \algref{alg:non-myopic} (with the oracle defined by Eq.~\eqref{eq:oracle:lattice})}
    \label{fig:app:lattice:adal}
  \end{subfigure}
  \caption{Teaching sequences generated by the myopic algorithm that greedily minimizes Eq.~\eqref{eq:objrank} and \algref{alg:non-myopic} (\adal) on a $4\times 4$ lattice. The learner's initial hypothesis is marked by orange, and the target is marked by green. The dark gray square represents the teaching example at the current time step, while light gray squares represent the previous teaching examples.}
  \label{fig:app:lattice}
\end{figure*}

\subsection{Proof of \lemref{lm:lattice}}
We now provide the details of \adal and \nonadal, based on which we prove \lemref{lm:lattice}.
\begin{algorithm}[t]
  \caption{\nonadal: the non-adaptive teaching algorithm for \lattice}\label{alg:nonadal}
  \begin{algorithmic}
    \STATE {\bf input:}
    $\Hypotheses$, $\ordering$, initial $\hypothesis_0$
    \STATE $P \leftarrow \text{NodesOnShortestPath}(\hinit, \hstar, \Hypotheses)$
    \STATE $T \leftarrow \text{NeighboringNodes}(P)$
    \STATE $Z \leftarrow (T\setminus P, P)$
    \STATE {\bf output:} Sequence of teaching examples $Z$
  \end{algorithmic}
\end{algorithm}

\paragraph{The oracle}
As we have briefly discussed in \secref{sec:algorithm}, we consider a distance-based oracle, which returns the first hypotheses that are closer %(measured by $\futurecostapprox(\hypothesis, \Hypotheses_t, \hstar)$) 
(measured by the length of the shortest path) to the target $\hstar$ than from $\hypothesis_t$. Formally, we define
\begin{align}\label{eq:oracle:lattice}
  \oracle(\hypothesis_t, \Hypotheses, \hstar) =
  & \{h'\in\Hypotheses:
    \forall h'' \in \Hypotheses, \orderingof{h''}{h_t} \leq \orderingof{h'}{h_t} \notag \\
  \implies &\dist(h'', \hstar) = \dist(h', \hstar) ~\vee~ \notag \\
  &\dist(h', \hstar) < \dist(h_t, \hstar) \leq \dist(h'', \hstar)\}
\end{align}
% \begin{align}\label{eq:oracle:lattice}
    %     \oracle(\hypothesis_t, \Hypotheses, \hstar) =
    %     & \{h'\in\Hypotheses:
            %             \forall h'' \in \Hypotheses, \orderingof{h''}{h_t} \leq \orderingof{h'}{h_t} \notag \\
    %     \implies &\futurecostapprox(\hypothesis'', \Hypotheses_t, \hstar) = \futurecostapprox(\hypothesis', \Hypotheses_t, \hstar) ~\vee~ \notag \\
    %           &\futurecostapprox(\hypothesis', \Hypotheses_t, \hstar) < \futurecostapprox(\hypothesis_t, \Hypotheses_t, \hstar) \leq \futurecostapprox(\hypothesis'', \Hypotheses_t, \hstar)\}
                  %   \end{align}

\paragraph{The adaptive teacher} Assume that the learner starts on a 2-d lattice, with all nodes unexplored. Then, at time step 0, since there is no other node blocking the way from $\hinit$ to $\hstar$, our oracle returns the adjacent nodes to $\hinit$ on the lattice in the direction of $\hstar$, as the intermediate target hypotheses. At time step $t$, if any of the adjacent nodes of $h_0$ in the opposite direction of $\hstar$ (henceforth are referred as ``bad neighbor'') is unexplored, the teacher will pick an example which explores/blocks it first, before exploring the current hypothesis itself. The reason is that,
\begin{itemize}
\item since the teacher progressively advances to the target hypothesis $\hstar$, it will never pick (random) teaching examples that explore all the adjacent nodes of the bad neighbors of $h_t$, before that bad neighboring node is explored. See \figref{fig:app:lattice:adal} as an example.
\item If a bad neighbor of $h_t$ has an unexplored neighbor other than $h_t$, then \adal will pick an example that explores the bad neighbor first before exploring the learner's current hypothesis (as going to the bad neighbor leads to lower gain in terms of the greedy objective, and hence we want to explore it before the learner jumps there).
\item If $h_t$ has no bad neighbor, then the teacher provides an example that explores $h_t$ itself, and the learner proceeds to the next intermediate target node.
\end{itemize}
From the above discussion, we know that the total number of nodes needs to be explored before reaching $\hstar$ is $((2 - 1) + 1)\cdot \dist(h_0, \hstar) = 2\dist(h_0, \hstar)$ (see \figref{fig:app:lattice:adal}, last plot). The same reasoning generalizes to $d-$dimensional lattice as well, where an adaptive teacher needs to explore the bad neighbors in $d$ directions, and progress in one direction at each round. Hence, the cost of \adal is of order $\bigO{d\cdot \dist(h_0, \hstar)}$.

\paragraph{The non-adaptive teacher} Our strategy for designing a non-adaptive neighbor follows closely from the adaptive strategy. Since the uncertainty of the teaching process comes from the learner randomly jumping to neighboring nodes of equal preference, we aim to pre-compute a set of teaching example that ensures the learner taking a deterministic path. Compared to the adaptive strategy which only explores ``bad'' neighbors, the non-adaptive teacher also has to explore ``good''neighbors to form a deterministic path from $\hinit$ to $\hstar$. In $d-$dimension, there are $2d$ directions in total, with one of them containing a good path. Therefore, the teacher needs at least $(2d-1)\dist(\hinit, \hstar)$, which finishes the proof of \lemref{lm:lattice}.
% The pseudocode for the non-adaptive teachen \nonadal is given in \algref{}

%%% Local Variables:
%%% mode: latex
%%% TeX-master: "main"
%%% End:
